# Supplementary material for: Learning Image-Conditioned Dynamics Models for Control of Under-actuated Legged Millirobots
Source: arXiv:1711.05253 source file (2018-03-30)
Supplement: Supplementary file 1 [file 07_appendix.tex]

\subsection{Differential Drive Baseline}

We present an instantiation of a common steering method used for robots with wheel or leg-like mechanisms on both sides, known as differential drive. In this control scheme, the turn rate $\omega_{\text{robot}}$ is proportional to the difference between left $\omega_l$ and right $\omega_r$ leg velocities. A differential drive controller assumes that the system behavior can be thought of as two wheels connected by a common axis: Here, moving the right wheel would turn the robot to the left, and moving the left wheel would turn the robot to the right. Note that this general idea of a difference in leg velocities translating to heading change of the entire system can be implemented in many ways, and we describe our implementation below merely as a guideline.

As described in Algorithm.~\ref{alg:dd}, our implementation of a differential drive controller uses robot heading, as well as perpendicular distance away from the desired path, in order to set velocity setpoints for each side of robot. In addition to standard heading control where the robot turns such that its heading matches the angle of the line, it also incorporates the perpendicular error metric to say that its heading should be more or less than the heading of the line, in order to actually move back toward the line. This controller outputs desired leg velocities at a rate of 10 Hz. To enable the realization of these leg velocities, we also implement a low-level PID controller that runs in the firmware at 1000 Hz. Encoder readings of the leg positions provide feedback, and the PID controller monitors proportional, integral, and derivative errors in order to output the PWM values required for achieving the desired leg velocities.

\begin{algorithm}
  \caption{A Differential Drive Algorithm\\for Trajectory Following}
  \label{alg:dd}
\begin{algorithmic}[1]
    \STATE \textbf{Inputs}: Current state $(x,y,z,\text{roll},\text{pitch},\text{yaw})$, \\ \hspace*{35pt}Desired waypoints $W= [w_0, w_1, \dots]$, \\ \hspace*{35pt}Controller parameters $f1$ and $f2$
    \STATE Line segment $L \leftarrow$ closest $[w_i,w_{i+1}]$ to $(x,y)$
    \STATE $d_{\text{line}} \leftarrow$ angle of $L$
    \STATE $p \leftarrow$ perpendicular distance of $(x, y)$ to line segment $L$
    \STATE \algorithmicif\ $(x,y)$ to right of $L$
    \STATE \algorithmicthen\ $d = d_{\text{line}} + f1*p$\
    \STATE \algorithmicelse\ $d = d_{\text{line}} - f1*p$\
    \STATE left leg velocity $\omega_l \leftarrow \omega_{\text{nom}} - d*f2$
    \STATE right leg velocity $\omega_r \leftarrow \omega_{\text{nom}} + d*f2$
    \STATE \textbf{Outputs}: leg PID velocity setpoints $\omega_l$ and $\omega_r$
\end{algorithmic}
\end{algorithm}

%%%%%%%%%%%%%%%%%%%%%%%%%%%%%%%%%%%%%%%%%%%%%%%%%%%%%%%%

\subsection{Choice of Action Abstraction}

Our model-based learning method allows users the freedom to vary the level of abstraction at which they would like to operate. Two options, which we illustrate in Fig.~\ref{fig:actionabstraction} as exhibiting comparable task performance, include setting direct motor PWM values and setting desired velocity setpoints.

Directly setting motor commands, instead of velocity setpoints, precludes the need to tune another layer of feedback control (i.e. lower-level PID controller) for calculating motor commands. The method of directly sending commands, however, encounters the problems involved with a lack of feedback loop. In the case of the VelociRoACH, a given PWM value can result in different amounts of leg movement, due to both variations in the battery level, as well as due to the leg kinematics leading to different forces at different stages of the leg rotation. At the same time, outputting desired velocities and then designing a lower-level PID controller to achieve those velocities involves an additional stage of parameter tuning, and one concern includes unpredictable behavior caused by not achieving the desired velocity within the time $\dt$ before the next setpoint is received. Each of these action abstraction options has pros and cons that manifest themselves differently on different systems. Thus, it is an enticing feature to have an algorithm easily adapt to the user's choice of action abstraction.

\begin{figure*}
    \centering
    \includegraphics[width=0.8\linewidth]{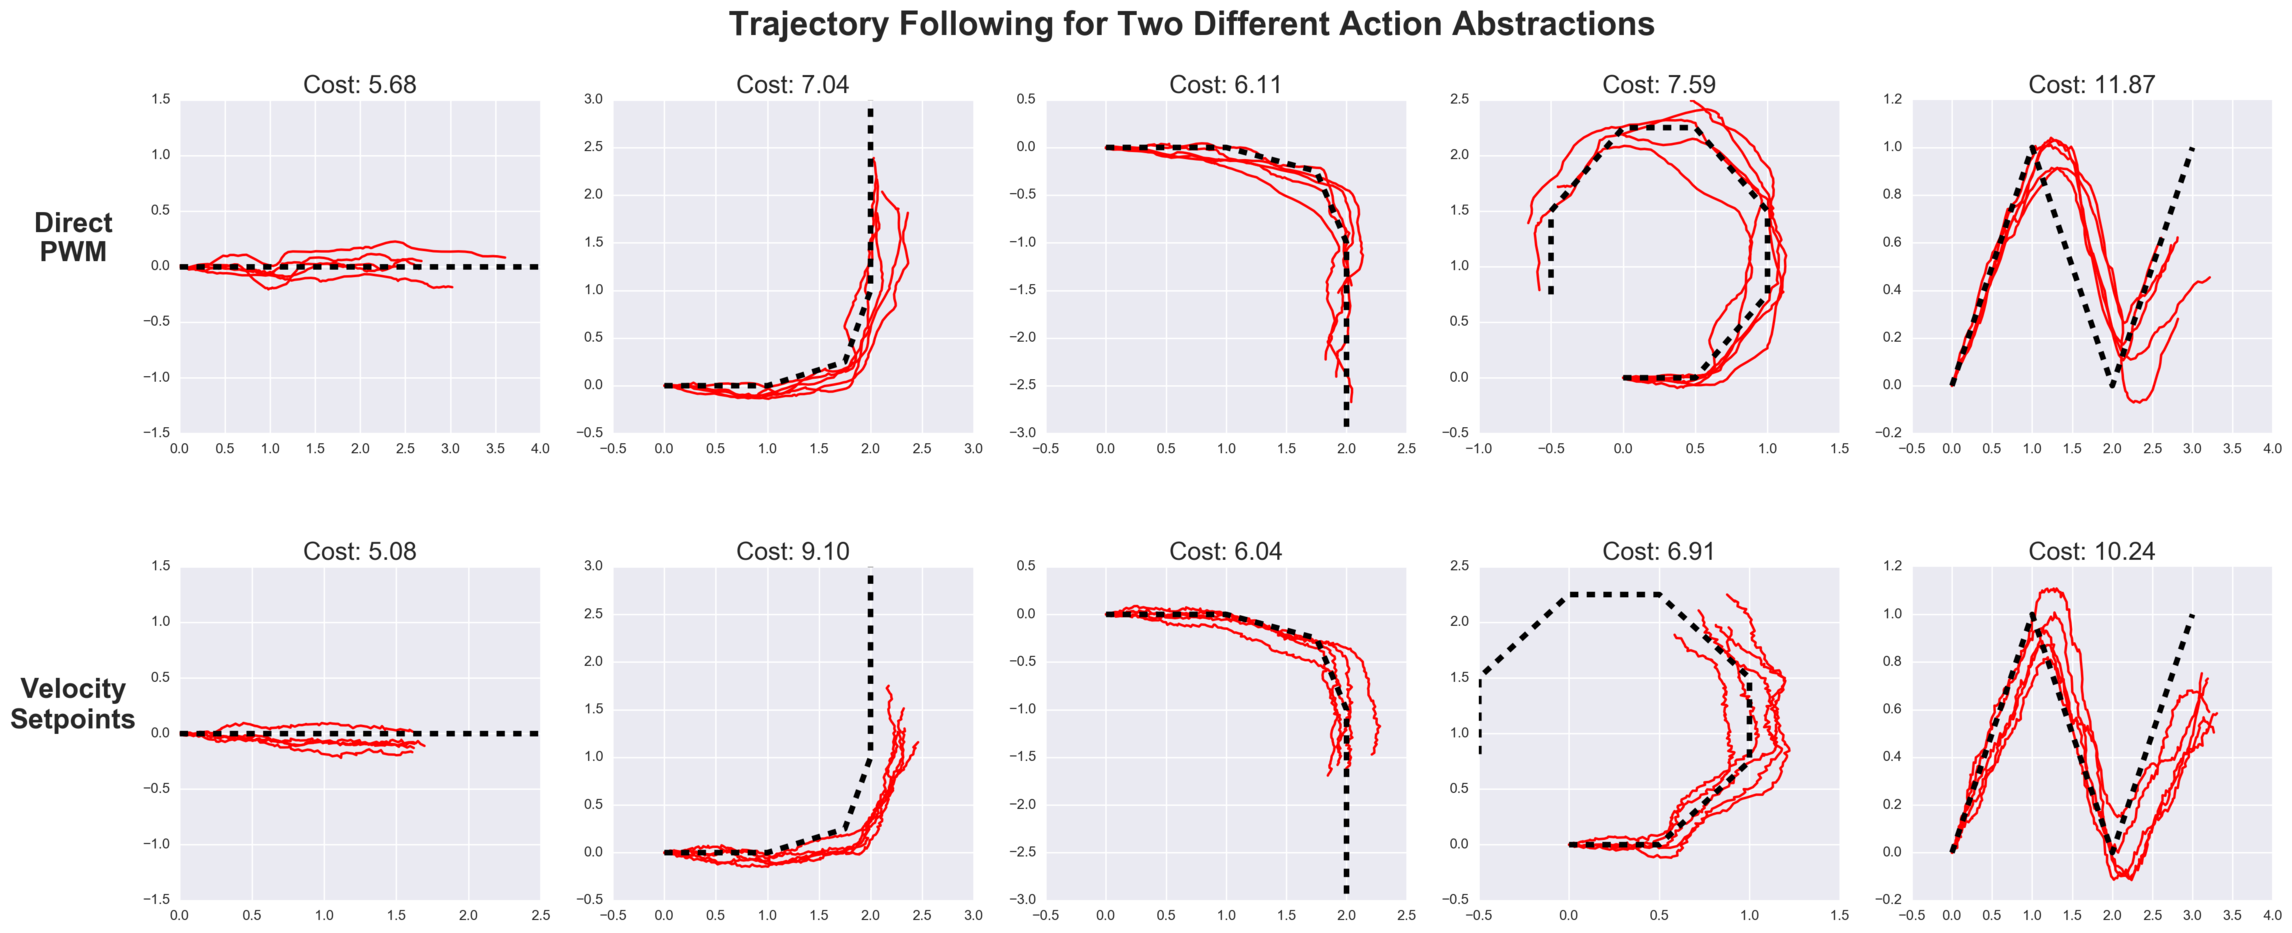}
    \caption{Trajectories executed by our model-based controller when the control outputs were (Top:) direct motor PWM values and (Bottom:) leg velocity setpoints, which a lower-level controller was tasked with achieving. Note that for each of these options, the corresponding dynamics model was trained using data where the $\ba_t$ represented the indicated choice of action abstraction.}
    \label{fig:actionabstraction}
\end{figure*}
